# Supplementary material for: Demystifying Oversmoothing in Attention-Based Graph Neural Networks
Source: arXiv:2305.16102 source file (2024-06-04)
Supplement: Supplementary file 1 [file appendices.tex]

\documentclass{article} % Not really important
\usepackage{pdfpages}
\begin{document}
\includepdf[pages={12-20}]{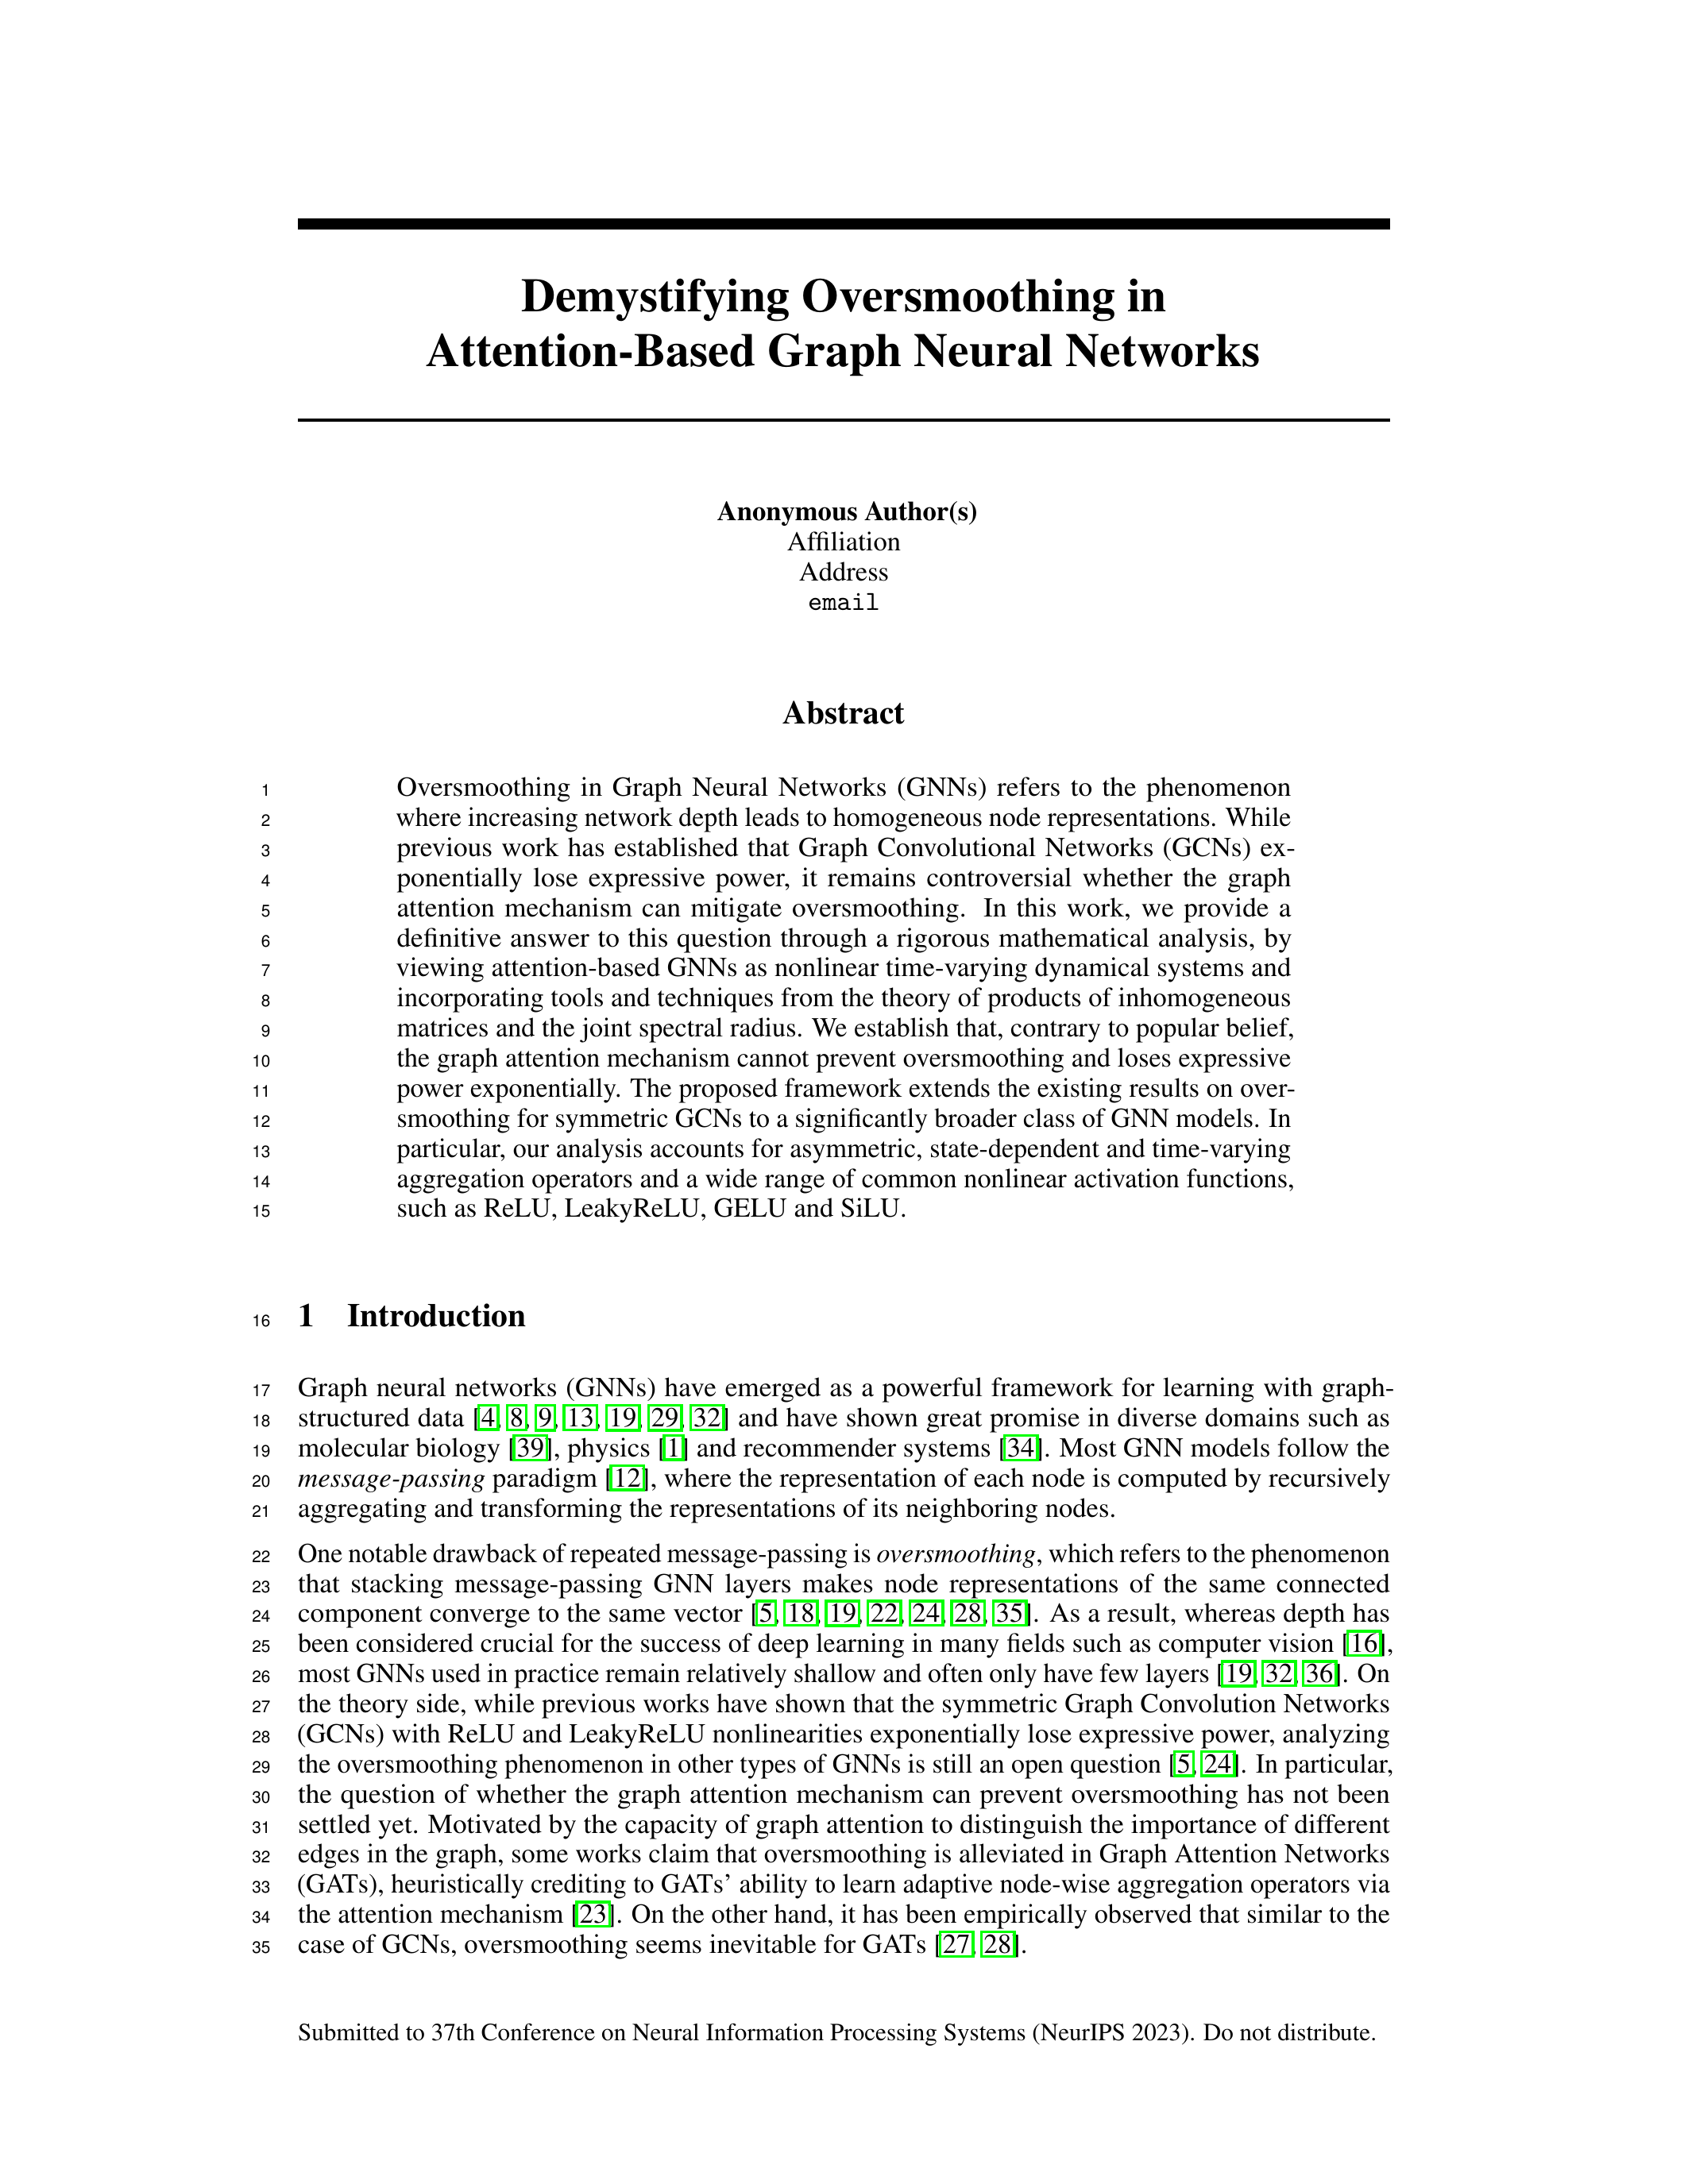}
\end{document}
